# Supplementary material for: Mitigating Participation Imbalance Bias in Asynchronous Federated Learning
Source: arXiv:2511.19066 source file (2025-11-24)
Supplement: Supplementary file 1 [file appendix_code.tex]

\section{Code }
