# Supplementary material for: Mitigating Participation Imbalance Bias in Asynchronous Federated Learning
Source: arXiv:2511.19066 source file (2025-11-24)
Supplement: Supplementary file 2 [file appendix_limitation.tex]

% \section{Limitation}\label{supp_sec:limit}

% While our proposed \shortname{} algorithm, including its \variantshortname{} variant, demonstrates superior performance in mitigating heterogeneity amplification and handling diverse delay settings in Asynchronous Federated Learning (AFL), a primary limitation relates to server-side resources.

% The core design of \shortname{} relies on aggregating gradient information from all clients for each global update. To achieve this, the server needs to maintain a cache or buffer to store the latest available gradient from every participating client. In scenarios with a very large number of clients, or when dealing with high-dimensional models where individual gradients are large, the memory requirement for this server-side buffer can become a significant practical consideration. Although this buffer is finite, its size scales with the number of clients and the model size.

% Appendix~\ref{supp_sec:8bit_quantization} explores the impact of 8-bit server-side gradient quantization on performance, primarily to demonstrate the robustness of \shortname{} to such compression techniques. This robustness is significant as compression also directly addresses the aforementioned server-side memory overhead. While the introduction of quantization/compression inherently involves certain considerations, such as potential minor impacts on convergence dynamics or numerical precision (which were not found to be detrimental in our current tests), these aspects deserve further exploration in diverse settings. The experimental results detailed in Appendix~\ref{supp_sec:8bit_quantization} show that 8-bit variations can achieve final performance comparable to the full-precision approach, indicating this robustness and highlighting quantization as a promising avenue for more scalable deployments of \shortname{}.

% Therefore, the primary limitation acknowledged is the server-side memory overhead required for full gradient aggregation, particularly in large-scale deployments. Future work might continue to explore more advanced compression techniques or adaptive buffering strategies to further optimize resource utilization without compromising the core benefits of the all-client aggregation approach.
